# Supplementary material for: Non-Stationary Latent Auto-Regressive Bandits
Source: arXiv:2402.03110 source file (2025-02-28)
Supplement: Supplementary file 1 [file bias_discussion.tex]

\section{Discussion on the Bias Term}
\label{sec_bias_disc}
% ref: https://pages.stern.nyu.edu/~dbackus/Identification/AndersonMoore_filtering_79.PDF
$|\lambda_{\max}(\Gamma)| < 1 \implies |\lambda_{\max}(\Gamma - \Gamma K C)| < 1$ \cite{anderson2005optimal}.
%%% BIAS LEMMA %%%
\begin{lemma}
\label{bounded_bias_lemma}
    [Bias Term Decays With Large $s$] If Assumption~\ref{assump_ar_process} holds, then the bias term 
    from Equation~\ref{eqn_bias}  $b_t(a, s) \rightarrow 0$ as $s \rightarrow \infty$ for all $a \in \mathcal{A}$.
\end{lemma}
\begin{proof}
    Recall that $    b_t(a, s) := \langle c_a, (\Gamma - \Gamma K C)^s \Tilde{z}_{t - s} \rangle$. Let $A = \Gamma - \Gamma K C \in \mathbb{R}^{k \times k}$. We first show that $|\lambda_{\max}(A)| < 1$.
    %%%%%%%
    First notice that $KC = (CPC^\top + V)^{-1}PC^\top C$. Since $PC^\top C$ is a rank 1 matrix, it has $k - 1$ eigenvalues equal to 0 and one non-zero eigenvalue, Let $\lambda_{\neq 0}$ denote the non-zero eigenvalue. Then:
    \begin{align*}
        \lambda_{\neq 0}(PC^\top C) = \sum_{i = 1}^{k} \lambda_i (PC^\top C) = \text{tr}(PC^\top C) = P_{11} \geq 0
    \end{align*}
    % which means that largest eigenvalue $\lambda_{\max}(PC^\top C) = P_{11}$.
    Also notice that $CPC^\top = P_{11}$. So $KC = \frac{PC^\top C}{P_{11} + V}$ has $k - 1$ eigenvalues that are $0$ and one eigenvalue equal to $\frac{P_{11}}{P_{11} + V} \in (0, 1)$. Furthermore, this implies that $I - KC$ has $k - 1$ eigenvalues that are equal to $1$ and one eigenvalue equal to $1 - \frac{P_{11}}{P_{11} + V} \in (0, 1)$.
    So $|\lambda_{\max}(I - KC)| < 1$.
    
    \alt{ANNA TODO: need to finish this.}
    \alt{Also need to use assumption that $|\lambda_{\max}(\Gamma)| < 1$}
    $A = \Gamma - \Gamma KC = \Gamma (I - KC)$.
    %%%%%%%
    
    Now we finish the proof.
    Any vector can be written as a linear combination of linearly independent eigenvectors. Therefore, we write $\Tilde{z}_{t - s}$ as a linear combination of eigenvectors of $A$. Let $\Tilde{z}_{t - s} = \sum_{i = 1}^{k} \alpha_i v_i$. Then:
    \begin{align*}
        A^s \Tilde{z}_{t - s} = \sum_{i = 1}^{k} \alpha_i A^s v_i = \sum_{i = 1}^{k} \alpha_i \lambda_i^s v_i
    \end{align*}
    Since $|\lambda_{\max}(A)| < 1$ as shown above, as $s \rightarrow \infty$, $\lambda_i^s \rightarrow 0$ for $i \in [k]$.
    This implies that $A^s \Tilde{z}_{t - s} \rightarrow \vec{0}$ as $s \rightarrow \infty$ because each $\alpha_i \lambda_i^s v_i \rightarrow \vec{0}$. So $b_t(a, s) \rightarrow 0$ as $s \rightarrow \infty$ for any $a \in \mathcal{A}$.
\end{proof}
