# Supplementary material for: Non-Stationary Latent Auto-Regressive Bandits
Source: arXiv:2402.03110 source file (2025-02-28)
Supplement: Supplementary file 2 [file e.tex]

\section{Method for Setting $k$}

\begin{figure*}[h!]
  \centering
  \subfigure[]{
    \includegraphics[width=0.48\textwidth]{icml2024/figs/ordered_lasso/ordered_lasso_d_5.pdf}
  }
  \subfigure[]{
    \includegraphics[width=0.48\textwidth]{icml2024/figs/ordered_lasso/ordered_lasso_d_10.pdf}
  }
  \caption{Ordered LASSO recovery on Toy Data. Ordered LASSO trained on $N = 100$ data-points. Toy data are i.i.d. draws from a standard normal.}
  \label{fig:ordered_lasso_toy}
\end{figure*}

In the setting where one has prior data (e.g., through an exploration phase), we offer a simple method of choosing a reasonable $k$ before running Algorithm~\ref{alg_known_k}. To learn a reasonable $k$ from prior data, first notice that if one chooses $k_0 > k$, then one can still learn an equivalent representation of the true parameter $\theta^* \in \mathbb{R}^{|\mathcal{A}|\cdot (2k|\mathcal{A}| + 1)}$ if the algorithm learns a $\hat{\theta} \in \mathbb{R}^{|\mathcal{A}|\cdot (2 k_0|\mathcal{A}| + 1)}$ where indices corresponding to $1, 2,...,k$ share the same parameters as $\theta^*$ and 0s otherwise. This motivates the approach of learning $k$ by 1) collecting data through an exploration phase, 2) learning a sparse representation for a high-dimensional state space from the collected data, and 3) uses the learned sparsity to commit to a value $\hat{k}$.
\cite{hao2020high}.
% Walter says in practice we should do soft commit: especially if you're are doing posterior sampling to just be strategic about your prior and set more shrinkage for larger order indices vs. smaller order indices.

\subsection{Ordered Lasso}
% alt: group lasso: https://group-lasso.readthedocs.io/en/latest/
To help learn more effectively, we incorporate that our problem has a natural order constraint on the parameters. Namely, we have the order constraint that features corresponding to past time-steps further away from $t$ (e.g., ones corresponding to $k_0$) should get less priority than time-steps closer to $t$.

Ordered Lasso \cite{suo2014ordered} is a variant of classic Lasso regression which performs Lasso but with an extra order constraint on the features. For simplicity of notation, the rest of the section refers to $d = |\mathcal{A}|\cdot (2 k_0|\mathcal{A}| + 1)$ as the dimension of the parameter. Assume for without loss of generality that features are rearranged in the desired order for our problem, as described above. Let the each dimension of the parameter we learn $\hat{\theta}$ be decomposed into $\hat{\theta}_j = \hat{\theta}_j^{+} - \hat{\theta}_j^{-}$ with $\hat{\theta}_j^{+}, \hat{\theta}_j^{-} \geq 0$ for all $j \in [d]$. Then Ordered Lasso (modified for our setting) has the following objective function:
\begin{align*}
    \min \;\; \frac{1}{2} \sum_{t = 1}^{T_0} \bigg(r_t - \sum_{j = 1}^{d} \hat{x}_{tj}(\hat{\theta}_j^{+} - \hat{\theta}_j^{-}) \bigg)^2 + \lambda \sum_{j = 1}^d (\hat{\theta}_j^{+} + \hat{\theta}_j^{-})
\end{align*}

subject to $\hat{\theta}_1^{+} \geq \hat{\theta}_2^{+} \geq \cdots \geq \hat{\theta}_d^{+} \geq 0$ and $\hat{\theta}_1^{-} \geq \hat{\theta}_2^{-} \geq \cdots \geq \hat{\theta}_d^{-} \geq 0$.

This decomposition is necessary to maintain that the objective is convex, while promoting sparse solutions and satisfying a soft order constraint.

\subsection{Experiments}
We first simulate an exploration or data collection phase where we randomly sample actions with equal probability. We consider multiple exploration lengths $T_0 = [50, 100, 500]$. We fix ground-truth $k = 2$ \alt{ANNA TODO: this may change} and latent noise $\sigma_z = 1$ and considered $k_0 = [2, 3, 5, 10]$.

Out of the 100 simulated trials, how many times do you select the correct $k$? How many times less? How many times selected greater?

Should have 3 tables
