# Supplementary material for: Non-Stationary Latent Auto-Regressive Bandits
Source: arXiv:2402.03110 source file (2025-02-28)
Supplement: Supplementary file 3 [file f.tex]

\section{Extension to Contextual Bandits}
Here we assume that $s_t$ is drawn from some distribution and is uncorrelated with $z_t$. We leave the correlated case to future work.
% note adversarial situations because we're motivated by mobile health

\begin{definition}
    \label{def_lar_extension}
    (Latent Auto-regressive Contextual Bandit) 
    Let $\mathcal{A} \subset \mathbb{N}$ be the action space. 
    The interaction between the environment and the agent is as follows. For every time-step $t \in [T]$:
    \begin{enumerate}
        \item The environment generates latent state $z_t \in \mathbb{R}$ of the form:
        \begin{equation}
        \label{ext_latent_state}
            z_t = \gamma_0 + \sum_{j = 1}^k \gamma_jz_{t - j} + \xi_t, \;\;\; \xi_t \overset{\text{i.i.d.}}{\sim} \mathcal{N}(0, \sigma_z^2)
        \end{equation}
        where $\gamma_0, \gamma_1, ..., \gamma_k \in \mathbb{R}$.
        \item The agent selects action $a_t \in \mathcal{A}$ observing state $s_t \in \mathbb{R}^d$ but without observing $z_t$.
        \item %%% LINEAR REWARD %%%
        The environment then generates reward $r_t$ given state $s_t$ and latent state $z_t$ and action $a_t$ is:
        \begin{equation}
        \label{ext_linear_reward}
            r_t = r(z_t, a_t) = \beta_0(a_t) + \beta_1(a_t) z_t + \sum_{i = 1}^d \beta_{i + 1}(a_t) (s_t)_i + \epsilon_t \;\;\; \epsilon_t \overset{\text{i.i.d.}}{\sim} \mathcal{N}(0, \sigma_r^2)
        \end{equation}
        where $\beta_0(a_t), \beta_1(a_t),...,\beta_{d + 1}(a_t) \in \mathbb{R}$ depends on the action $a_t$.
        \item The agent observes $r_t$.
    \end{enumerate}
\end{definition}

\begin{lemma}
\label{extension_of_rewrds}
\textbf{(Alternative Form of Latent AR Contextual Bandit)} Suppose latent state $z_t$ evolves in an $k$-order autoregressive process of Equation~\ref{latent_state} with some initial state $z_0$. Let $s_{1},...,s_{t- 1}$, $a_1,..,a_{t - 1}$, and $r_1,..,r_{t - 1}$ be the observed states, actions and rewards up to time $t$. Then given state $s_t$, for fixed $a$, $r_t$ defined in Equation~\ref{linear_reward} has the form:
\begin{equation}
\label{eqn_ext_general_rewards}
    r_{t}(a) = \Tilde{\beta_0}(a) + \beta_1(a) \sum_{j = 1}^{k} \gamma_j \frac{r_{t - j} - \beta_0(a_{t - j}) - \epsilon_{t - j}}{\beta_1(a_{t - j})} + \sum_{i = 1}^d \beta_{i + 1}(a) (s_t)_i + e_t(a)
\end{equation}
where
\begin{equation}
\label{ext_general_bias}\Tilde{\beta_0}(a) = \beta_0(a)+ \beta_1(a)\gamma_0
\end{equation}
and
\begin{equation}
\label{ext_general_errors}
e_t(a) = \epsilon_t + \beta_1(a)\xi_t
\end{equation}
\end{lemma}

\begin{proof}
\alt{ANNA TODO}
\end{proof}
