# Supplementary material for: Non-Stationary Latent Auto-Regressive Bandits
Source: arXiv:2402.03110 source file (2025-02-28)
Supplement: Supplementary file 4 [file latent_ar_oracle.tex]

\section{Latent AR Oracle}
In this section, we derive the update and action-selection procedures of the latent AR oracle defined in Section~\ref{sec_regret_def}. Recall that the oracle does not observe the realization of latent state $z_t$. Instead, the oracle knows the ground-truth parameter $\theta^*$ which includes $\gamma_0,..,\gamma_k, \mu_a, c_a\; \forall a \in \mathcal{A}$ from Equations~\ref{latent_state}, \ref{linear_reward}, noise variances $\sigma_z^2, \sigma_r^2$, and all realizations of past rewards from all actions, $R_{1: t - 1}$.

The key idea is to first notice that the oracle uses the Kalman filter with $|\mathcal{A}|$ reward observations per time step from the linear Gauss-Markov model. This is in contrast to the agent which only observes a single reward per time step. Recall the state dynamics in the linear Gauss-Markov model corresponding to the latent AR bandit is:
% The linear Gauss-Markov model associated with the oracle is:

\begin{align}
    Z_t = \Gamma Z_{t - 1} + W_t, \;\;\; W_t \sim \mathcal{N}_{k + 1}(\mathbf{0}, Q)
\end{align}
where
\begin{align*}
    \Gamma = \begin{bmatrix}
        1 & 0 & 0 &\cdots & 0 \\
        \gamma_0 & \gamma_1 & \gamma_{2} & \cdots & \gamma_k \\
        0 & 1 & 0 & \cdots & 0 \\
        \vdots & \vdots & \vdots & \vdots & \vdots \\
        0 & 0 & \cdots &  1 & 0
    \end{bmatrix} \in \mathbb{R}^{k + 1 \times k + 1}, \;\;\;
    Z_{t - 1} = \begin{bmatrix}
        1 \\
        z_{t - 1} \\
        z_{t - 2} \\
        \vdots \\
        z_{t - k}
    \end{bmatrix} \in \mathbb{R}^{k + 1}, \;\;\;
    W_t = \begin{bmatrix}
        0 \\
        \xi_t \\
        0 \\
        \vdots \\
        0
    \end{bmatrix} \in \mathbb{R}^{k + 1}
\end{align*}

At time $t - 1$, the oracle obtains observation vector $X_{t - 1}$ where:
\begin{align}
    X_{t - 1} = C Z_{t - 1} + \phi_{t - 1}, \;\; \phi_{t - 1} \sim \mathcal{N}_{|\mathcal{A}|}(\mathbf{0}, R_{\phi} = \sigma_r^2 I)
\end{align}
where
\begin{align*}
    X_{t - 1} = \begin{bmatrix}
        r_{t - 1}(1) \\
        r_{t - 1}(2) \\
        \vdots \\
        r_{t - 1}(|\mathcal{A}|)
    \end{bmatrix} \in \mathbb{R}^{|\mathcal{A}|}, \;\;\;
    C = \begin{bmatrix}
        \mu_1 & c_1 & 0 &\cdots & 0 \\
        \mu_2 & c_2 & 0 &\cdots & 0 \\
        \vdots & \vdots & \vdots &  & \vdots \\
        \mu_{|\mathcal{A}|} & c_{|\mathcal{A}|} & 0 & \cdots & 0
    \end{bmatrix} \in \mathbb{R}^{|\mathcal{A}| \times k + 1}, \;\;\;
    \phi_{t - 1} = \begin{bmatrix}
        \epsilon_{t - 1}(1) \\
        \epsilon_{t - 1}(2) \\
        \vdots \\
        \epsilon_{t - 1}(|\mathcal{A}|)
    \end{bmatrix} \in \mathbb{R}^{k + 1}
\end{align*}

% \begin{align}
%     R_t = \mathbf{\beta} Z_t + E_t
% \end{align}
% where
% \begin{align*}
%     \beta = \begin{bmatrix}
%     \beta_0(1) & \beta_1(1) & 0 & \cdots & 0 \\
%     \beta_0(2) & \beta_1(2) & 0 & \cdots & 0 \\
%     \vdots & \vdots  & \vdots & \vdots  & \vdots \\
%     \beta_0(|\mathcal{A}|) & \beta_1(|\mathcal{A}|) & 0 & \cdots & 0
% \end{bmatrix} \in \mathbb{R}^{|\mathcal{A}| \times k + 1}, \;\;\;
%     E_t = \begin{bmatrix}
%         \epsilon_t(1) \\
%         \epsilon_t(2) \\
%         \vdots \\
%         \epsilon_t(|\mathcal{A}|)
%     \end{bmatrix} \in \mathbb{R}^{|\mathcal{A}|}
% \end{align*}

To simplify notation, let $\Tilde{Z}_{t}$ be the oracle's estimator for $Z_t$ where $\Tilde{Z}_{t} = \Tilde{Z}_{t | t - 1} = \mathbb{E}[Z_t | R_{1:t - 1}; \theta^*]$ and let $\Tilde{r}_t(a) = \mu_a + c_a^\top\Tilde{z}_t$ be the oracle's estimator for the mean reward. Since we assume that $(\Gamma, C)$ are observable (i.e., can be estimated using only the outputs for all possible state evolutions) and $Q$ is positive definite, then the Kalman gain matrix $K_t$ converges. Therefore, using the steady-state Kalman filter for $\Tilde{Z}_{t}$, we can re-write the reward (Equation~\ref{linear_reward}) using terms up to the past $s > 0$ time steps \citep{gornet2022stochastic}:

\begin{align}
    r_t(a) = G_a \mathbf{X}_t + \langle c_a, (\Gamma - \Gamma K C)^s \Tilde{Z}_{t - s} \rangle + \varepsilon_{a; t} 
\end{align}

where
\begin{align}
    G_a := \begin{bmatrix}
    c_a^\top(\Gamma - \Gamma K C)^{s - 1} \Gamma K & \cdots & c_a^\top \Gamma K & \mu_a
    \end{bmatrix}
    \in \mathbb{R}^{1 \times (|\mathcal{A}| \cdot s + 1)}
\end{align}
\begin{align}
    \mathbf{X}_t := \begin{bmatrix}
    X_{t - s}^\top & \cdots & X_{t - 1}^\top & 1
    \end{bmatrix}
    \in \mathbb{R}^{(|\mathcal{A}| \cdot s + 1) \times 1}
\end{align}
\begin{align}
    \varepsilon_{a; t} := r_t(a) - \Tilde{r}_t(a) = \langle c_a, z_t - \Tilde{z}_t \rangle + \epsilon_t(a) \sim \mathcal{N}(0, c_a^\top P c_a + \sigma_r^2)
\end{align}
\begin{align}
    K = PC^\top(CPC^\top + R_{\phi})^{-1}
\end{align}
\begin{align}
    P = \Gamma P \Gamma^\top + Q - \Gamma P C^\top (CPC^\top + R_{\phi})^{-1}CP\Gamma^\top
\end{align}

% and $\Sigma_{t | j}^O = \mathbb{E}[(Z_t - Z_{t | j}^O)(Z_t - Z_{t | j}^O)^\top]$. 

% Using the standard formula for multivariate normal, we can derive the update and action-selection procedures as follows:

% \textbf{Update}
% \begin{align}
%     z_{t | t}^O = z_{t | t - 1}^O + \Sigma_{t | t - 1}^O \beta^\top (\beta \Sigma_{t | t - 1}^O \beta^\top + E)^{-1}(R_t - \beta z_{t | t - 1}^O)
% \end{align}
% \begin{align}
%     \Sigma_{t | t}^O = \Sigma_{t | t - 1}^O - \Sigma_{t | t - 1}^O \beta^\top (\beta \Sigma_{t | t - 1}^O \beta^\top + E)^{-1} \beta \Sigma_{t | t - 1}^O
% \end{align}
% where $E = \text{Var}(E_t) = \sigma_r^2 I_{|\mathcal{A}|}$

% \textbf{Action-Selection}
% \begin{align}
%     z_{t | t - 1}^O = A z_{t - 1 | t - 1}^O
% \end{align}
% \begin{align}
%     \Sigma_{t | t - 1}^O = A \Sigma_{t - 1 | t - 1}^O A^\top + W
% \end{align}
% where $W = \text{Var}(W_t)$

\textbf{Notes on Regret}

Assume for simplicity that both oracle and agent know $\theta^*$, $\mathcal{A} = \{0, 1\}$, and the reward for action $a$ at time $t$ is $r_t(a) = \beta(a) z_t + \epsilon_t(a)$. However, oracle and agent never observe the realization of $z_t$.

The following regret is originally defined in this paper: https://arxiv.org/pdf/2205.01970 on pg. 10.
\begin{align*}
    \text{Regret}_{\text{LAR}}(T) =
    \sum_{t = 1}^T  \mathbb{E} \bigg[\underset{a \in \mathcal{A}}{\max} \; \mathbb{E}[r_t(a) | R_{1:t - 1}; \theta^*]
    - \mathbb{E}[r_t(a_t) | \mathcal{H}_{t - 1}] \bigg]
\end{align*}

\begin{align*}
    = \sum_{t = 1}^T  \beta(a_t^{O}) z_t - \beta(a_t) z_t
\end{align*}
where $a_t^O = \arg \max_{\{0, 1\}} \beta(a) z^{O}_{t | t - 1}$ is the action selected by the oracle where $z^{O}_{t | t - 1}$ is informed by reward realizations of \textit{all} actions $R_{1: t - 1}$ and $a_t = \arg \max_{\{0, 1\}} \beta(a) z^{\text{agent}}_{t | t - 1}$ is the action selected by the agent where $z^{\text{agent}}_{t | t - 1}$ is informed by only reward realizations of actions it took.

Notice that $\Delta_t = 0$ if the oracle and the agent select the same action. Otherwise:
\begin{align*}
    \Delta_t = \mathbb{E}[\beta(a_t^O) z_t - \beta(a_t) z_t] = |(\beta(1) - \beta(0)) z_t| \cdot \text{Pr}(a_t^O \neq a_t)
\end{align*}

Assuming that the first term $|(\beta(1) - \beta(0)) z_t|$ does not trivially go to 0, we want $\text{Pr}(a_t^O \neq a_t) \rightarrow 0$ as $t \rightarrow \infty$. 

Intuition: If gap between $(\beta(1) - \beta(0))$ is large OR variance of agent's estimator compared to oracle's z value is small then you're fine. But Anna is having a hard time writing the math for it...
