# Supplementary material for: Non-Stationary Latent Auto-Regressive Bandits
Source: arXiv:2402.03110 source file (2025-02-28)
Supplement: Supplementary file 6 [file additional_figs.tex]

\section{Additional Figures}
\label{app_additional_graphs}
