# Supplementary material for: Non-Stationary Latent Auto-Regressive Bandits
Source: arXiv:2402.03110 source file (2025-02-28)
Supplement: Supplementary file 9 [file lds_reduction.tex]

\section{Exact Forms for Lemma~\ref{linear_dynamic_system}}
\label{exact_forms_lds_lemma}
